# Supplementary material for: Experimental Evidence that Zn Impurities Pin Pair-Density-Wave Order in La$_{2-x}$Ba$_x$CuO$_4$
Source: arXiv:2010.00610 source file (2020-12-21)
Supplement: Supplementary file 1 [file LBCO_Zn_Supplemental_Material.pdf]

# Supplementary Material: Experimental Evidence that Zn Pins Pair-Density-Wave Order in $La_{2-x}Ba_xCuO_4$

P. M. Lozano,[1,2] G. D. Gu,[1] J. M. Tranquada,[1] and Qiang Li[1,2]
[1]*Condensed Matter Physics & Materials Science Division, Brookhaven National Laboratory, Upton, New York 11973-5000, USA*
[2]*Department of Physics and Astronomy, Stony Brook University, Stony Brook, NY 11794-3800, USA*

(Dated: September 21, 2020)

## I. DATA REPRODUCIBILITY AND INFLUENCE OF IMPERFECT CRYSTAL ALIGNMENT ON IN-PLANE RESISTIVITY

In Fig. S1, the in-plane ($\rho_{ab}$) and c-axis ($\rho_c$) resistivities are plotted as a function of temperature from 2 to 40 Kelvin at a few selected magnetic fields (0, 2, and 14 Tesla) applied along the c-axis. For clarity, the normalized data are shown that were taken in four single crystals side-by-side cut from the same slab, two (D2-1 and D2-2) for $\rho_{ab}$, and two (D1-1 and D1-2) for $\rho_c$ measurements. An extended temperature view of the same data at zero field for all four samples (unnormalized) are presented in Fig. S2. The insets to Figure S2 show the resistivity measurement configuration sketches and a picture of a studied sample with contact wires attached. The shaded green areas in the sketches are the pre-deposited silver contact pads that are annealed at elevated temperature for a short time [1] to produce a low contact resistance ($< 1\Omega$). Gold wires are attached to the contact pads with silver paint. Narrow voltage contact channels are around the outer perimeter of the entire cross-section, while the current contacts are made at the end of the crystals to ensure uniform current flow and voltage sensing. The grid scale in the picture is 1 mm. $\rho_{ab}$ shows a metallic behavior above superconducting transition up to 300K, while a semiconductor-like behavior is observed for $\rho_c$, consistent with the previous measurement of other LBCO single crystals [1]. A modest jump in $\rho_{ab}$ occurs near 32.5K, and it is associated with a first-order structure transition.

The overall features of the temperature and magnetic field dependence of resistivity for all six samples (four for $\rho_{ab}$ and two for $\rho_c$) we characterized are very similar. The only noticeable differences are in the appearance of in-plane ($\rho_{ab}$) resistivity humps around 22.5 K below the onset of 2D superconducting transition, due to the imperfection of crystal alignment between current flow direction and the ab-plane. This hump feature is well-known in the transport measurement of extremely anisotropic superconductors, such as this Zn-doped LBCO with very high normal state resistivity anisotropic ratio that grows as temperatures decreases. In our samples, $\rho_c/\rho_{ab}$ reaches a value of $\sim 1.5 \times 10^4$ above superconducting transition. A misaligned angle of $0.7^\circ \sim \sqrt{\frac{\rho_{ab}}{\rho_c}}$ in our samples would produce the residual c-axis resistivity component being comparable to the value of $\rho_{ab}$ when measuring $\rho_{ab}$ in such a misaligned crystal [1, 2]. Thus, it is emphasized here that an imperfectly aligned crystals with a misaligned angle higher than $1^\circ$ in these Zn doped LBCO crystals can lead to the measured "in-plane resistivity" being overwhelmed by the residual c-axis resistance component, thus masking the onset of 2D superconductivity. It is instructive to demonstrate here that the magnitude of the hump in $\rho_{ab}$ near 22.5 K can be used for assessing the actual misalignment in the measured single crystals, being $0.29^\circ$ for sample D2-2 and $0.54^\circ$ for sample D2-1. Small crystal misalignment has much less effect on the value of $\rho_c$, which is evident in the $\rho_c$(T) curves for D1-1 and D1-2, as shown in Fig. S2a.

## II. MEAN FIELD TRANSITION TEMPERATURES $T^c_{\rm R}$, $T^{ab}_{FS}$, AND $T^c_{FS}$

Mean field transition temperatures are determined using the steepest slope approach, except those specifically stated otherwise in the main text. In Fig. S3, we show the temperature dependence of the in-plane $\rho_{ab}$ and its derivatives $d\rho_{ab}/dT$ of a Zn-doped LBCO single crystal (D2-2) at 0, 1, 6, and 14T magnetic field applied parallel to the c-axis. The temperatures, $T^c_{\rm R}$, at the maximum $d\rho_{ab}/dT$ (depicted as stars) are taken as the mean-field superconducting transition temperature. The same procedures are applied for determining $T^{ab}_{FS}$ and $T^c_{FS}$ from susceptibility vs T curves.

## III. INITIAL MAGNETIZATION

The initial magnetization measurements for $H//$c and //ab, after the sample was zero-field cooled to 2K, are presented in Fig. S4. Full superconducting shielding for $H//$ab collapses at around 2.0 mT, with rapid penetration of magnetic field into the ab-planes. For $H//$c, full shielding was observed at applied field up to 30 mT, after which the superconducting shielding weakens gradually, as magnetic field penetrates into the sample. The peak penetration field is over 100 mT, a typical behavior expected of a 3D type II superconductor in mixed state.

[1] Q. Li, M. Hücker, G. D. Gu, A. M. Tsvelik, and J. M. Tranquada, Two-dimensional superconducting fluctuations in stripe-ordered $la_{1.875}ba_{0.125}cuo_4$, Phys. Rev. Lett. **99**, 067001 (2007).

[2] Y. Li, J. Terzic, P. G. Baity, D. Popović, G. D. Gu, Q. Li, A. M. Tsvelik, and J. M. Tranquada, Tuning from failed superconductor to failed insulator with magnetic field, Science Advances **5**, 10.1126/sciadv.aav7686 (2019).

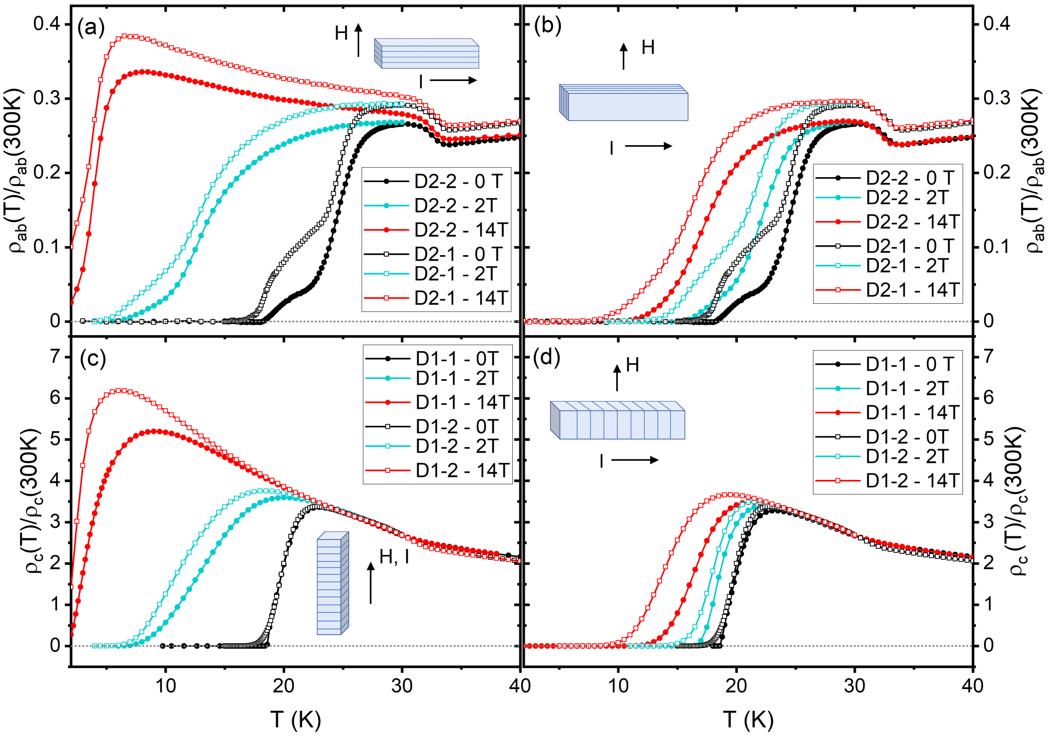


FIG. S1. Temperature dependence of $\rho_{ab}$ (samples D2-1 and D2-2) and $\rho_c$ (samples D1-1 and D1-2), normalized to their values at 300K, of Zn doped LBCO in a few selected magnetic fields applied parallel (a, c) or perpendicular (b, d) to the c-axis, respectively. Orientations of the crystals' ab-plane with respect to the applied current and magnetic field are sketched in the insets.

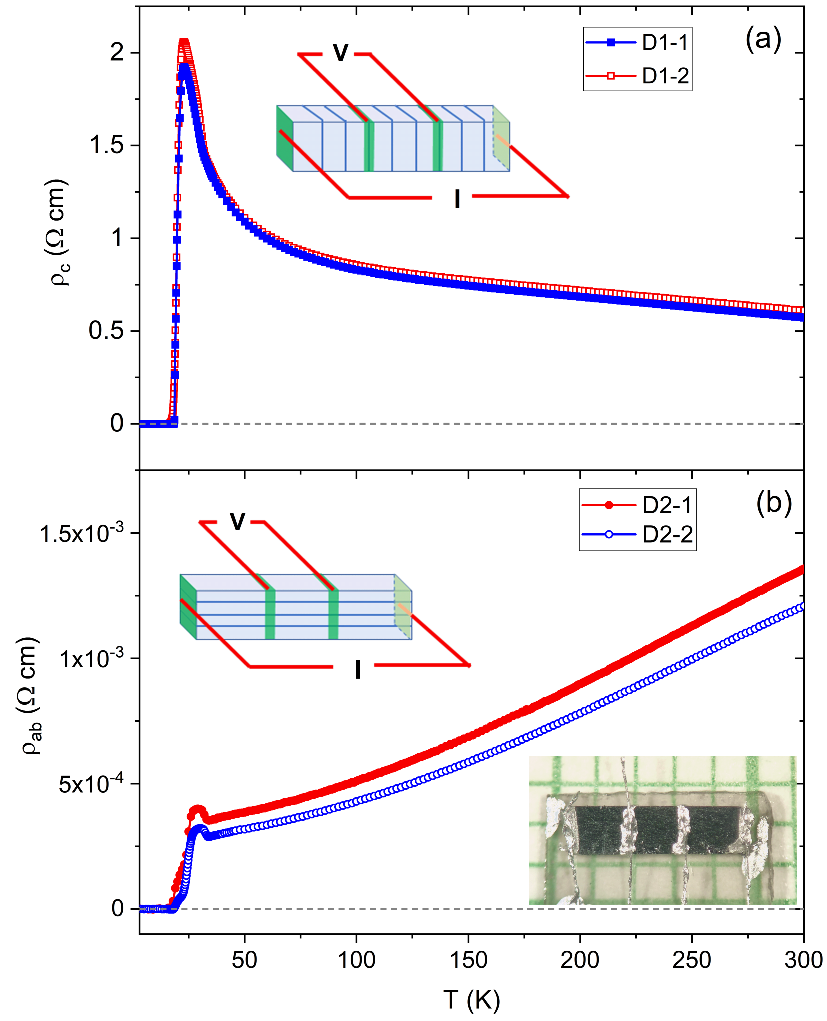


FIG. S2. Temperature dependence of the zero field $\rho_{ab}$ and $\rho_c$ for samples D1-1, D1-2, D2-1, and D2-2. The insets show the resistivity measurement configuration sketches and the picture of a sample with contact wires attached, where the grid scale is 1 mm. The shaded green areas in the sketches are the pre-deposited silver contact pads. Narrow voltage contact channels are around the outer perimeter of the entire cross-section, while the current contacts are made at the end of the crystals to ensure uniform current flow and voltage sensing.

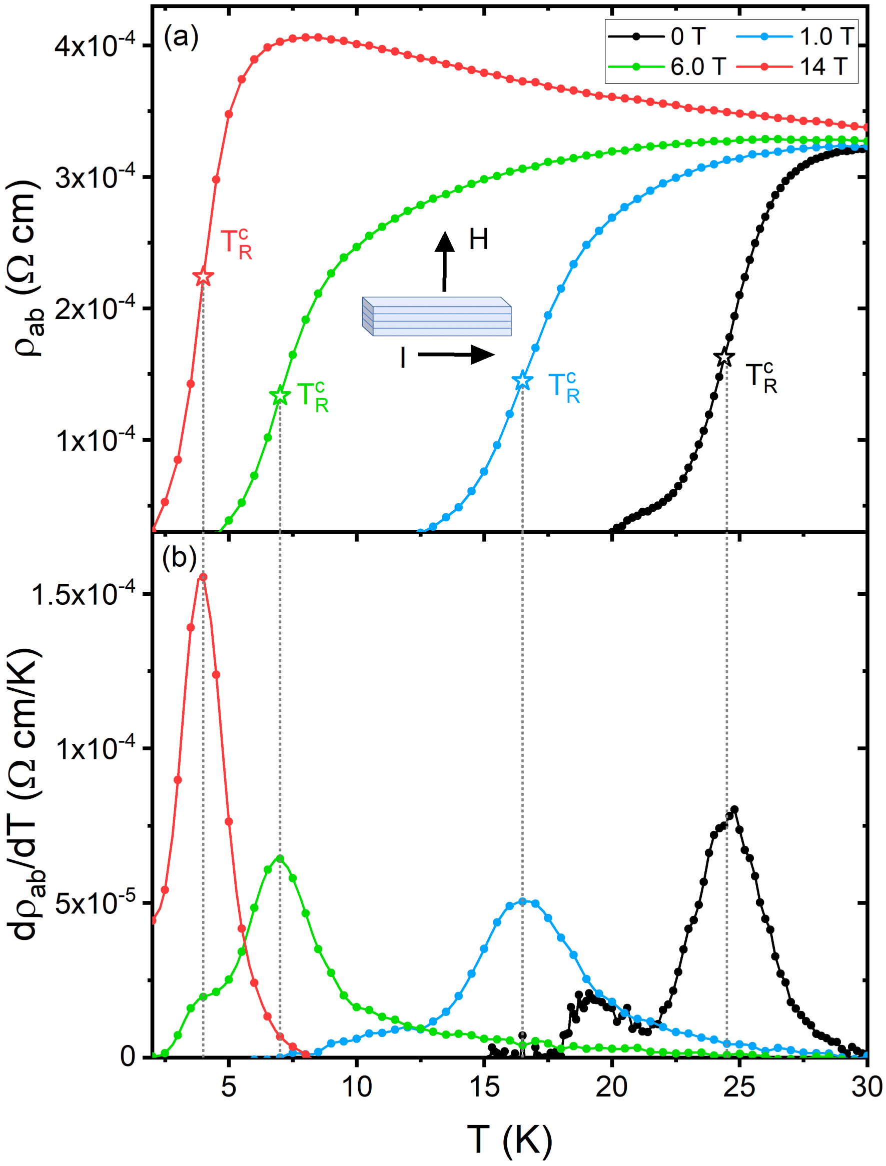


FIG. S3. Temperature dependence of $\rho_{ab}$ and its derivatives $d\rho_{ab}/dT$ of a Zn-doped LBCO single crystal at 0, 1, 6, and 14T magnetic fields applied parallel to the c-axis. The temperatures $T_{\rm R}^{c}$ at the maximum $d\rho_{ab}/dT$, depicted as stars, are the mean-field superconducting transition temperatures.

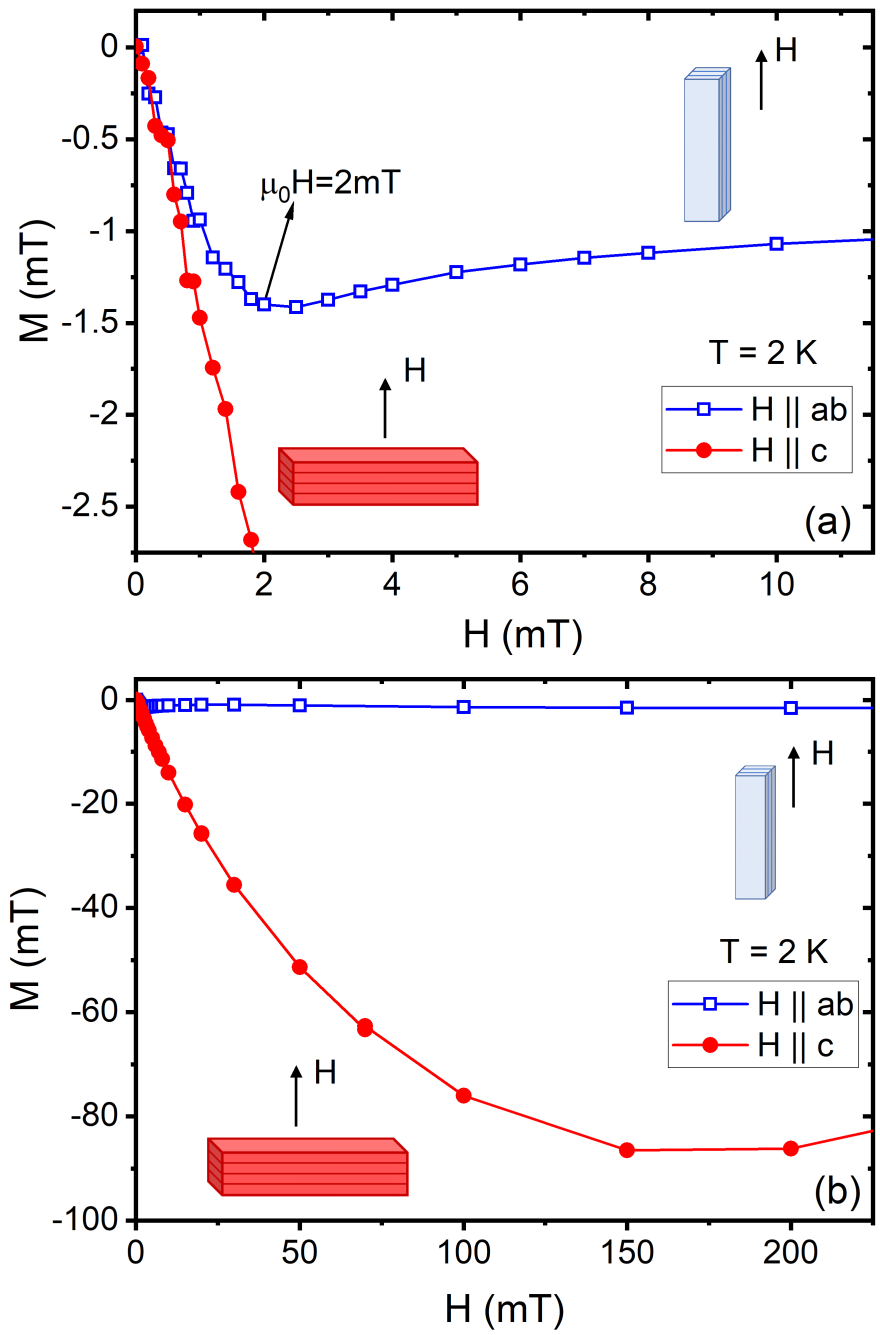


FIG. S4. The initial magnetization for $H//$c and //ab, after the sample was zero-field cooled to 2K. (a) is an expanded view of the same data in (b) at the low field region.
